# Supplementary material for: Improving the Inference of Topic Models via Infinite Latent State Replications
Source: arXiv:2301.12974 source file (2023-01-25)
Supplement: Supplementary file 1 [file appendix.tex]

\section{Hyper-parameter sensitivity}

%%%%Nex experiments
CGS is sensitive to the hyper-parameter choices. Hence, we study the predictive perplexity as a function of the hyper-parameter settings. In this experiment, we vary $\alpha$ and $\beta$ from $0.01$ to $0.5$ and we set $K=25$.  In addition, we let the methods run for 10000 iterations to guarantee a fair assessment. Table \ref{tab:hyperparameters}  presents the results when running the experiments on movielens.

\begin{table}[b]
  \caption{Predictive perplexity across different $\alpha$ and $\beta$ hyper-parameter values on movielens. Best result per dataset is in boldface and the second best is underlined. RCA is highlighted with gray.}
  \label{tab:hyperparameters}
  \centering
  \begin{tabular}{l@l^l^l^l^l}
    \toprule
    $\alpha$ \textbackslash ~$\beta$ & 0.01 &  0.05 &  0.10 &  0.25 &  0.50\\
    \midrule
	        \multirow{2}*{0.01}  & 981.7 & 958.4 & 944.6 & 940.2 & 934.6\\
    & \rowstyle{\cellcolor{hcolor}}910.7 & 906.8 & 904.7 & 901.8 & 899.7\\   
            \multirow{2}*{0.05}  & 957.9 & 932.0 & 922.6 & 921.1 & 920.8\\
    & \rowstyle{\cellcolor{hcolor}}906.8 & 904.2 & 902.6 & 900.3 & 898.3\\
            \multirow{2}*{0.10}  & 945.0 & 924.8 & 920.6 & 911.2 & 910.4\\
    & \rowstyle{\cellcolor{hcolor}}904.3 & 902.1 & 901.0 & 899.3 & 897.4\\
            \multirow{2}*{0.25}  & 937.1 & 918.2 & 911.2 & 908.1 & 906.3\\
    & \rowstyle{\cellcolor{hcolor}}900.6 & 899.0 & 898.0 & 897.3 & 895.7\\
            \multirow{2}*{0.50}  & 925.1 & 913.6 & 909.3 & 904.7 & 905.2\\
    & \rowstyle{\cellcolor{hcolor}}898.2 & 896.8 & 895.9 & 895.3 & 896.3\\
    \bottomrule
  \end{tabular}
\end{table}

Results show a consistent improvement of RCA over LDA-CGS. For any hyper-parameter setting, RCA yields a better predictive perplexity. In particular, we observe that the setting that yields the worst result for RCA is comparable with the setting that yields the best perplexity for LDA-CGS. Furthermore, we observe that LDA-CGS is more sensitive to the hyper-parameter choice having a range in perplexity of 76. Even for the same value of alpha or beta, the range in perplexity is as large as 56.6. Our proposed method  instead has a difference in perplexity of 15.4 across all hyper-parameter settings. In the worst case fixing alpha or beta has a difference in perplexity of at most 11.
